# Supplementary material for: The worst of both worlds: A comparative analysis of errors in learning from data in psychology and machine learning
Source: arXiv:2203.06498 source file (2022-06-02)
Supplement: Supplementary file 1 [file old4_appendix.tex]

\appendix
\section{Methods}
Our analysis is informed by explicit collecting and reading papers on reproducibility and replication concerns with an eye toward comparing psychology and AI and ML over the course of a little over a year. We used note-taking and qualitative thematic analysis approaches led by the first author but with input from other authors. While drafting the paper, the first author conferred with various researchers in machine learning, including presenting to an industry machine learning lab. 
Our analysis is also heavily informed by our longer term interests and commitments to methodological reform across the social sciences and AI and ML. %The author team includes 




\section{Background}
%\subsection{Bias-variance trade off}

%{\bf I recommend removing this section as it's just saying something that's been said in many other places by others, so it's just an invitation for us to get some detail wrong which will make us look bad! --- AG}

%The classical bias variance trade off describes how given a statistical model, the variance of the parameter estimated across samples (i.e., the error from sensitivity to fluctuations in the training set) can be reduced by increasing the bias in the estimated parameters as defined classically as the expected error conditional on the unknown true parameter value. \jessica{add equations} The expected generalization error for a learning problem can be expressed as the sum of the squared bias, variance, and irreducible error using the bias-variance decomposition. A modeler’s goal is to find the best balance between underfitting and overfitting the data, such that the learned model is sufficiently expressive of the true data generating process while avoiding hallucinating parameter relationships from irreducible or sampling error characterizing the data used for learning. Comparing the typical model used in social psychology to that of modern machine learning and particularly deep learning, the goal of causal attribution leads to prioritization of simpler models, often selected and fit with an eye toward minimizing bias. On the other hand, machine learning systems can use more than ten orders of magnitude more parameters than a typical regression specified by a psychologist, and tend to be designed with greater emphasis on controlling variance than bias [explain why complexity is more tolerable in the predictive setting - see eg Efron 2020 Prediction~\cite{efron2020prediction}] 

%While the classical bias variance decomposition has provided a formalism for understanding key differences between the causal attribution versus predictive modeling paradigm, in the last several years, attempts to understand the behavior of some (overparameterized) deep learning models have directly challenged the classical understanding~\cite{belkin2018overfitting} [Nakkiran et al 2019, [others]]. Though researchers were aware of of the potential to train models whose parameters exceeded the number of training instances following a breakthrough by Hinton and colleagues~\cite{krizhevsky2012imagenet}, only in the last couple years have theorists conceptualized and proposed general explanations for the phenomena. Belkin et al.~\cite{belkin2019reconciling} showed that given a fixed training sample size $n$, plotting risk curves as a function of an approximate measure of a model’s complexity (number of parameters $N$) show that as N increases, risk minimizes initially, increases until training data are perfectly explained $(N=n)$, then decreases again. Others extended the results, showing the influence of the number of training epochs and proposing a general complexity measure for models [Nakkiran et al. 2019]. A ``universal law of robustness”~\cite{bubeck2021universal} shows that for any parameterized function class and a broader class of data distributions, overparameterization by a factor of $d$ representing the dimensionality of the data is necessary for smooth interpolation, or in other words, that there is a tradeoff between the size of a model by number of parameters and its robustness as measured by Lipschitz constant. Such findings have led to beliefs among some in the field that ML has potential to expand mathematical understanding in ways that render the surface analogy of mimicking human brains through artificial intelligence irrelevant~\cite{sejnowski2020unreasonable}, and resulted in proposals of the discovery of a new field of mathematical analysis of deep learning~\cite{berner2021modern}.  

\subsection{Bridging causal and predictive modeling}
Yarkoni and Westfall~\cite{yarkoni2017choosing} construe the adaptive data analyses paradigm common in psychology as a ``relatively low-bias but high-variance approach,” in that it returns nearly any pattern that might exist in a dataset but at the cost of many spurious results. They characterize p-hacking as a form of ``procedural overfitting” that takes place prior to or in parallel with model estimation, and argue for the adoption of ML techniques over current standards in psychology research, including large observational datasets, cross-validation and model selection, and regularization. Hildebrandt~\cite{hildebrandt2018preregistration} argues that selection of performance metrics is analogous to p-hacking in social science, and calls for pre-registration of ML models. Hofman et al.~\cite{hofman2017prediction} similarly point out undisclosed degrees of freedom in predictive modeling as researchers translate research questions into computational tasks including task, data set, model, and performance metric selection. They argue that approaches to evaluating predictive accuracy require standardization, comparison to relevant baselines and defining best possible performance and that predictive accuracy and interpretability must be recognized as complements when evaluating explanations. More recently, Hofman et al.~\cite{hofman2021integrating} propose a quadrant framework of (1) descriptive research, (2) tests of causal claims (explanatory modeling), (3) tests of passive predictive claims (predictive modeling), and (e4) tests of claims for both causality and predictive accuracy. They suggest more methodological focus on generalization to quadrant 4, more sharing of methods across quadrants, and adoption of methods that combine predictive and exploratory modeling, as well as clearer labeling of contributions by quadrant and granularity of claims, and standardization of open science practices across social and computer science.  %Our work is complementary: by summarizing important threats to learning in testing of causal claims (i.e., social psychology) versus passive predictive claims (i.e., machine learning), and reflecting on underlying sources of epistemological uncertainty that both motivate and challenge notions of threats, our framework points to places where critiques are related and AI and ML researchers can learn from one another despite their different goals.  

Analogies between concerns in AI and ML and concerns around replication in the social sciences have been made in motivating reproducibility interventions like checklists and dataset and model summaries~\cite{pineau2021improving,gebru2021datasheets,mitchell2019model} at AI and ML venues. %Writing for the popular press, Hutson~\cite{hutson2018ai} accused AI and ML methods of being ``black boxes'' that require engineers to use trial and error in the absence of a deep understanding of how performance achievements are obtained. 
Pineau and colleagues~\cite{pineau2019iclr,pineau2021improving,haibe2020transparency,khetarpal2018re} describe  
how problems related to open science, such as clear descriptions of methods and open data and code, threaten research in machine learning and reinforcement learning in particular.  
Bell and Kampman~\cite{bell2021perspectives} argue that psychology provides a useful comparison for ML because ``both fields study complex systems with surprising emergent behaviors,'' and suggest greater use of pre-defined methods and preregistration in ML and changes to culture and incentives. % Liao et al.~\cite{liao2021we} examine evaluations in ML, dividing issues into problems with internal validity (e.g., bad baselines) and external validity (e.g., bad generalization). 
%\jessica{add more that make explicit analogies between repl crisis and ML}


\subsection{Evidence of irreproducibility in ML}
Evidence of the irreproducibility of psychology studies is documented as part of various replication projects~\cite{nosek2012scientific,camerer2018evaluating,klein2018many}.
We summarize more recent examples of evidence of the irreproducibility of machine learning research. 

Gorman and Kjensmo~\cite{gorman2019we} survey 400 papers at top AI conferences, analyzing potential for reproducibility based on features of the papers like well documented goals and procedures for methods and experiments. They find that none exhibit ``experiment reproducibility'' (the use of the same implementation of the method and the same data produces the same results), ``data reproducibility'' (the use of a different implementation of the method and the same data produces the same results) or ``methods reproducibility'' (the use of a different implementation of the method and a different dataset produces the same results). 



Several reproducibility challenges have been organized alongside ML conferences which attempted to independently verify empirical claims from published papers. These include the 2018 and 2019 ICLR reproducibility challenges \cite{iclr2018reproducibility, iclr2019reproducibility, pineau2019iclr} and the 2019 NeurIPS reproducibility challenge \cite{neurips2019reproducibility,pineau2021improving}, which were followed by more general reproducibility challenges for top ML conferences in 2020 and 2021 \cite{ML2020reproducibility,ML2021reproducibility}. These reproducibility challenges have highlighted the cultural and technical difficulties in ensuring the reproducibility of ML research, even in top ML conferences \cite{pineau2021improving}, but also authors' seeming willingness to submit code and reviewers willingness to engage with it~\cite{pineau2021improving}.

% \jessica{finish and add cites}


Kapoor and Narayanan~\cite{kapoor2021irreproducible} attempted to reproduce papers that adopted ML methods in a subfield of Political Science and found that all papers claiming the superior performance of ML models compared to baseline Logistic Regression models failed to reproduce due to data leakage. 

Raff et al.~\cite{raff2019step} attempted to independently reproduce results from 255 papers and found they could reproduce at least 75\% of the reported results in only 63.5\% of the papers. %When authors were responsive, 85\% of results could be reproduced, but when they weren't only 4\% could. 

 




%\jessica{add summaries of: Colberg and Todd 2016}
 
%Taking a more meta-level critical perspective, some researchers have pointed to problems with dominant narratives or practices of reform in social sciences and ML. Some have critiqued assumptions in ``normative'' reform arguments addressed at psychologists, such as the assumption that replication can be used to discriminate true effects~\cite{devezer2020case} and that preregistration addresses the fundamental issues that lead to a lack of replicability in social science~\cite{szollosi2019preregistration,szollosi2021arrested}. Philosophers have argued that assumptions about objectivity, credibility, and the nature of psychological phenomena underlying perspectives on the replication crisis should be more carefully reviewed in seeking solutions~\cite{morawski2019replication}, and that seemingly ``irrational'' aspects  of science like epistemic diversity~\cite{cheng2000strong} or scientists’ personal motivations may benefit the enterprise overall~\cite{zollman2018credit}. In ML, researchers have pointed to problematic assumptions or restricted viewpoints in how researchers engage with concepts of bias and fairness in critical themed work (e.g.,~\cite{blodgett2020language}). Our work also motivates further reflection on challenges that may be raised to the epistemological basis of proposed reforms despite their presumed practical benefits. 


  
\section{Supplemental details on specific threats to learning }


\subsection{Data collection and preparation}
\textbf{Social psychology.} Positive predictive value (PPV) denotes the probability that an observed effect which passes a significance threshold actually reflects a “true effect” as given by the equation $PPV = (1-\beta) R / ((1-\beta) R + \alpha)$, where $1-\beta$ is the power of the study, $R$ is the prior odds that a probed effect is non-null among the effects being probed, and $\alpha$ is the nominal significance level~\cite{button2013power}. Button et al.~\cite{button2013power} use an example of trying to detect an association with effect size equivalent to a 1.2 odds ratio using an (underpowered) study that can detect that size effect only 20\% of the time. Sampling variation and random error in measurements of the variables and outcomes of interest will mean that any individual study may find an effect less than or greater than 1.2, but the underpowered design will not enable detecting effects of 1.2 or less in most cases. 

%Related to misunderstandings of power, back in 1966 Bakan~\cite{bakan1966} described how authors seemed to assume that studies that produce negative results must have lack sensitivity to detect the effect, while any single positive study must be a well-executed sensitive experiment~\cite{bakan1966} as cited in \cite{szucs2017null}.

Meng~\cite{meng2018statistical} discusses how in the absence of random sampling, estimation error does not decreases with the square root of the sample size, counter to intuitions derived from simple statistical theory.
For a dataset of size $n$, "the difference between the sample average $\bar{X}_{n}$ and the population average $\bar{X}_{N}$ is the product of three terms: (1) a data quality measure, $\rho_{R,X}$ the correlation between $X_{j}$ and the response/recording indicator $R_{j}$; (2) a data quantity measure, $\sqrt{(N-n)/n}$, where $N$ is the population size; and (3) a
problem difficulty measure, $\sigma_{X}$, the standard deviation of $X$."
Decomposing error in this way implies that without probabilistic sampling, estimation error approaches a constant and does not decline like $\frac{1}{\sqrt{n}}$.  Hence, the possibility for bias should be accounted for in combining estimates, even for studies with large sample size.


\textbf{Machine learning.} Related to measurement bias, ``historical bias'' is said to result from structural inequalities in the world~\cite{suresh2021framework}, such as the fact that racial minorities and women with equivalent qualifications were less likely to be admitted to a medical school in the past data that an automated admissions algorithm is trained on (\cite{lowry1988blot} as cited in~\cite{barocas2016big}). Historical bias is said to lead to biased learning if not explicitly modeled as a source of error in capturing an intended construct (e.g., applicant quality).

\subsection{Model representation}

\textbf{Social psychology.} 
In defining a small world of model configurations through choice of a representation, there is inherent uncertainty in knowing whether the true model is in the small world of configurations under consideration. An M-closed model space refers to one that contains the true process \cite{bernardo1994}. However, true DGPs corresponding to human behaviors of interest are likely to be conceptualizable but too complicated to write explicitly (M-complete model space) or not even conceptualizable (M-open model space). When it can’t be assumed that the true model is in the observational model, for inferences to be meaningful the observational model must faithfully approximate the structure of the true data generating process in a way that serves the inference goals of the research~\cite{prior2017}. 

Beyond structural misspecification, researchers also tend to overlook the potential for a single observational model to reasonably approximate many true data generating processes~\cite{prior2017}. For example, linear models with assumptions of Gaussian variation in the variables are a type of first order approximation that might describe a wide range of generating processes, not just the one the researcher might imagine. %though researchers often overlook the potential for multiplicity and assume that the true DGP they conceive is uniquely identified by the model representation. 

Psychology researchers are said to misinterpret goodness of fit indicators like $R^2$ as describing predictive validity of the specific parameter estimates obtained from inference, when in reality it estimates the average proportional reduction in squared error if the functional form were repeatedly fit to new samples~\cite{yarkoni2017choosing}. 

%One way that simple models can be well motivated under smaller $N$ because the observations will be only weakly informative, such that any differences between a true data generating process and the inferred process are not possible to resolve. At larger $N$, it becomes possible to resolve such differences, which can then render the asymptotic limit irrelevant, as it is based on assumptions of the model space containing the true data generating process \cite{prior2017}.

\textbf{Machine learning.}
Bias from representations that make false assumptions about the target function is tolerated and even beneficial in ML, as when the misspecified model obtains higher accuracy than a well specified one by learning more efficiently from the available data. For example, Domingos’~\cite{domingos2012few} demonstrates how a naive Bayes classifier achieves higher accuracy than a rule-based learner despite a rule-based true data generating process for certain sample sizes. 

Poor calibration of uncertainty statements under distribution shift is addressed by Ovadia et al.~\cite{ovadia2019can}, who show how the quality of commonly used predictive uncertainty metrics in deep learning including negative log-likelihood, Brier score, and expected calibration error (ECE) degrades consistently with increasing dataset shift. 
Approaches to distribution-free uncertainty quantification, such as conformal prediction~\cite{vovk2005algorithmic,angelopoulos2020uncertainty}, represent uncertainty post-hoc and extrinsic to the selected model representation, so long as it provides a heuristic measure of uncertainty (such as pseudo-probabilities representing model confidence assigned by using softmax in the final layer of a deep neural net). However, the usefulness (i.e., the width) of uncertainty intervals generated this way ultimately still depends on the information in the heuristic measure and the generating probability distribution~\cite{shafer2008tutorial}. 

Adversarial robustness has largely been framed as a positive property of a model, but recently some have questioned its predominant treatment as value-free, as it may conflict with other desirable properties like suppressing dissent~\cite{albert2020politics} or giving those affected by predictions actionable recourse to change their label~\cite{ustun2019actionable}. 

Geirhos et al.~\cite{geirhos2020shortcut} associate shortcut learning with a failure to capture necessary complexity: situations where the inductive bias that arises from some combination of model representation, data, objective function and optimization approach tends toward models based on small numbers of simple features, while the human assumption is that the object of complex tasks like object recognition should rely on combinations of features derived from different attributes. Other perspectives, e.g., in NLP~\cite{gardner2021competency}, express a similar view. 
Shortcut learning motivates greater acknowledgment of correlations between features and how models progressively differentiate task structure by learning certain features first~\cite{arjovsky2019invariant,arpit2017closer,valle2018deep,hermann2020shapes}. Different takes on shortcut learning emphasize slightly different aspects of the true DGP that are not captured, including a lack of learning of reusable mechanisms, which tend to capture structure in the environment~\cite{scholkopf2012causal} or a failure to capture causal structure in particular~\cite{arjovsky2019invariant,scholkopf2012causal}.


D’Amour et al.~\cite{d2020underspecification} motivate underspecification of the learning pipeline, and specifically, failure to represent which inductive biases are more desirable to constrain learning, as a distinct but related issue from structural failure due to spurious features in the training data that are not associated with the label in other settings (i.e., distribution shift). %Underspecification occurs when predictors with equivalent performance on i.i.d. data from the same distribution as training degrade non-uniformly in performance when probed along practically relevant dimensions~\cite{d2020underspecification}. 
Underspecification captures observations about predictive multiplicity~\cite{marx2020predictive,fisher2019all}, i.e., the fact that a single learning problem specification can support many near optimal solutions that differ along dimensions like fairness or interpretability~\cite{ross2017neural}. 
Underspecification can be detected when a predictor’s performance on stress tests–referring to tests that empirically probe a model’s inductive biases along dimensions that are considered practically relevant–is sensitive to arbitrary choices for preserving the performance of predictors on i.i.d. data, like the choice of random seed or step size schedules chosen for trainability. In contrast to structurally induced failure (i.e., concept drift) which degrades performance similarly across predictors, variation of predictor performance indicates meaningful differences between predictors from a human perspective that is not made explicit in the learning pipeline. The idea of a pipeline being underspecified can be analogized to the limitations in social psychology around explicitly capturing prior knowledge in modeling, though in this case the missing prior concerns inductive biases that a human deems credible.

A recently demonstrated problem related to fine-tuning is that the appropriate values of hyperparameters tuned for foundation models cannot be inferred from testing in-distribution accuracy alone~\cite{wortsman2021robust}. More aggressively fine tuning a model has been shown to improve in-distribution performance but reduce out-of-dist\-ri\-bu\-tion performance in turn~\cite{wortsman2021robust}, making uncertainty about the distribution at deployment time a fundamental challenge to selecting among model configurations.  


Deep learning research has increasingly converged in architectures through the focus on foundational models. In addition to dataset deficiencies (Section~\ref{sec:data}), one risk is that a move toward huge models in terms of parameter space (up to billions as in GPT-3~\cite{brown2020language} or GShard~\cite{lepikhin2020gshard}, and even trillions as in Switch-C~\cite{fedus2021switch}), and fact that on some benchmarks performance continues to improve with increases to the number of hyperparameters~\cite{devlin2018bert} negatively impacts the environment~\cite{bender2021dangers,strubell2020energy}. When large models are generative, such as in the case of large language models that can be used to write human-like texts, the model representations are critiqued as not capable of capturing actual language understanding~\cite{bender2021dangers}, for example because they rely on spurious cues~\cite{le2020adversarial,niven2019probing}, and have access to form but not meaning via unlabeled training data~\cite{bender2020climbing}. However, a human faced with a generated text may mistake the speech for intentional speech by an understanding agent~\cite{bender2021dangers}. A convergence of research interest on large models brings opportunity costs over other types of representations and learning processes that could be explored~\cite{bender2021dangers}.  

\subsection{Model selection and evaluation}
%Common optimizers such as Adagrad and Adam are adaptive, and hyperparameters such as learning rate can vary for each training parameter to decrease the chances the optimizer gets stuck in undesirable local minima. However, adaptive descent produces a new complex dynamical system each time it is run, introducing complexity that makes it difficult to know whether better performance from one optimizer over another on a particular learning problem reliably signals a superior optimizer. 

%\jessica{Prabhat et al. (2019) show how hard it is to get a deterministic algorithm to runon a GPU. Even when succeeding on one computer, the results are completely different, butstill deterministic, on another computer.}

\textbf{Machine Learning.}
To demonstrate the problems that arise when data transformation steps are not carefully considered in designing the cross validation procedure, Neunhoeffer and Sternberg~\cite{neunhoeffer2019cross} provide an example based on down-sampling an input data set to balance the dependent variable prior to cross-validation. This procedure can lead to underestimates of error if the balancing is also applied to the fold used for testing in cross validation as iterations, as error estimates will then not describe situations like the input data where they are unbalanced. 

Large benchmark datasets are often thought to encompass artifacts and concepts in sufficient generality to capture their essence across contexts~\cite{raji2021ai}. While claims to universality appear plausible due to the large size of modern machine learning datasets, Raji et al.~\cite{raji2021ai} show that these datasets often lack culturally specific context, and the same dataset created in a different cultural context would emphasize different objects and concepts. Claims of universality of the performance of ML models across cultures can result in overoptimism about their applicability across contexts.

Related to the potential for performance claims to be invalidated by real world testing, a real-world study on the performance of a clinical risk prediction model for recommending chemotherapy found that when the model disagreed with human clinical judgement, using the model’s outcome resulted in worse outcomes when the model suggested chemotherapy, but the model could help prevent false positives in human clinical judgement~\cite{cardoso201670} as cited in~\cite{malik2020hierarchy}. Studies evaluating ML models in real world systems can offer insights into scenarios where ML models work well and where they don’t. In addition, real world testing on the population of interest can also offer realistic performance evaluations of ML models.

%Analogous to power concerns in social psych, critics point to high sampling error relative to signal in performance comparisons, where reporting point estimates of accuracy on test sets or in human model-validation studies ignores the presence of sampling error~\cite{card2020little}. 

Some evidence suggests adherence use of appropriate baselines and quantification of uncertainty in performance comparisons in ML is worsening over time~\cite{marie2021scientific}.


\subsection{Communication of claims}
\textbf{Social psychology.}
Another basic form of communication failure occurs in psychology research when authors fail to explain what types of uncertainty constructs they are reporting (e.g., 95\% CIs, prediction intervals, or standard error intervals)~\cite{krzywinski2013error}, or omit or downplay graphical communication of uncertainty, believing it will make the message of a chart to ambiguous or confusing to readers~\cite{hullman2019authors}. 

\textbf{Machine learning.} 
While 87\% of authors of 173 papers included in the NeurIPS 2019 reproduciblity challenge saw value in clearly defining metrics and statistics, 36\% judged error bars not applicable~\cite{pineau2021improving}.  

Another issue is the insertion of "spurious theorems" into a paper to increase the perceived legitimacy of the results, without serving to demonstrate the main claims of the paper~\cite{lipton2019research}. An overreliance on theory has been observed in other subfields of computer science as well~\cite{herley2017sok,newell2007computer}. % [Mitzenmacher: blog1, blog2; Herley 2017, Newell and Simon, 1976].

%\subsection{Culture}
%\textbf{SP.} 
%\textbf{ML.}
%As example of the implications of research developed ML models that ignore best practices in a domain, in medical imaging, Nagendran et al.~\cite{nagendran2020artificial} find a high risk of bias in a systematic review of deep learning models developed for medical imaging. Similarly, Roberts et al.~\cite{roberts2021common} find that all deep learning models that predict COVID-19 using chest radiography images suffer from validity issues. 
